# Supplementary material for: Safe and Stable Control Synthesis for Uncertain System Models via Distributionally Robust Optimization
Source: arXiv:2210.01341 source file (2023-03-16)
Supplement: Supplementary file 1 [file Appendix.tex]

\section{Appendix}
\label{sec: appendix}

\subsection{Constraint Function for Multi-Input Case}
In this section we consider a more general case:
\begin{equation}\label{mimo: dynamics}
	\dot{\bfx} = f(\bfx) + A_1 \bfxi_1 + [g(\bfx) + A_2 \bfxi_2] \bfu, \ \ \bfx \in \bbR^n
\end{equation}
where $\bfu \in \calU \subseteq \bbR^m, \ m \geq 2$. Define $\underline{\bfxi} = [\bfxi_1 \ vec(\bfxi_2)]^T, \ \underline{\bfxi} \in \Xi$. 
~\\
The constraint function becomes:
\begin{equation}\label{mimo: ACC_constraint}
\begin{aligned}
	&\bfF(\bfu,\underline{\bfxi}) = \\
	&\left[ \begin{matrix}
	-\mathcal{L}_{f(\bfx) + A_1 \bfxi_1} h({\bfx}) - \mathcal{L}_{g(\bfx) + A_2 \bfxi_2} h(\bfx) \bfu - \gamma h(\bfx) \\
	\mathcal{L}_{f(\bfx) + A_1 \bfxi_1} V(\bfx) + \mathcal{L}_{g(\bfx) + A_2 \bfxi_2} V(\bfx) \bfu + \epsilon V(\bfx) - \delta
	\end{matrix} \right]
\end{aligned}
\end{equation} 
We could rewrite the uncertainty and constraints as the following form:
\begin{equation}
\bfF(\bfu,\underline{\bfxi})^T :=\begin{matrix} \underline{\bfu} \left[ \tilde{A}_1  \ \  \tilde{A}_2 \right] \underline{\bfxi} \end{matrix} + \begin{matrix} \left[ b_1(\bfu) \ \ b_2(\bfu) \right] \end{matrix}, \ \ \underline{\bfxi} \in \Xi
\end{equation}
where $\underline{\bfu} = [1 \ \ \bfu^T]^T$,
\begin{equation}
\begin{aligned}
	&\tilde{A}_1
	=	
	\left[ \begin{matrix}
	-\frac{\partial{h(\bfx)}}{{\partial{\bfx}}}A_1 && \bf0 \\
	\bf0 && -I_m \otimes \frac{\partial{h(\bfx)}}{{\partial{\bfx}}}A_2
	\end{matrix} \right], \\
	&\tilde{A}_2
	=	
	\left[ \begin{matrix}
	\frac{\partial{V({\bfx})}}{{\partial{\bfx}}}A_1 && \bf0 \\
	\bf0 && I_m \otimes \frac{\partial{V({\bfx})}}{{\partial{\bfx}}}A_2
	\end{matrix} \right], \\
	&b_1(\bfu) = -\frac{\partial{h(\bfx)}}{{\partial{\bfx}}} ( f(\bfx) + g(\bfx) \bfu ) - \gamma h(\bfx), \\
	&b_2(\bfu) = \frac{\partial{V({\bfx})}}{{\partial{\bfx}}} ( f(\bfx) + g(\bfx) \bfu ) + \epsilon V(\bfx) - \delta
\end{aligned} \nonumber
\end{equation}
\subsection{Convex Reformulation as Mix-integer QP}
In equation \eqref{eq: CBF_Convex_Reformulation_Final} we solve the following problem:
\begin{equation}
\label{eq: inf_t}
\min_{t \in \mathbb{R}} \frac{1}{N} \sum_{i=1}^{N} (-\textit{CBC}(\bfx,\ubfu,\bfxi_i) + t)_+ - t \epsilon. 
\end{equation}
The optimal $t$ is given by: $t = \textit{CBC}(\bfx,\ubfu,\bfxi_k), \ k = \lceil N\epsilon \rceil$.
To ease notation, we write $\textit{CBC}(\bfx,\ubfu,\bfxi_i)$ as $\textit{CBC}_i$. In order to get the close-form solution of equation \eqref{eq: inf_t}, we made an assumption that $\textit{CBC}_i$ is in ascending order: $\textit{CBC}_i \leq \textit{CBC}_j, \ i \leq j$. However, to further reformulate \eqref{eq: CBF_Convex_Reformulation_Final} in to a mix-integer quadratic-problem, we need to further assume that: $\textit{CBC}_i \neq \textit{CBC}_j, \ i \neq j$. \par
First, we consider a special case of \eqref{eq: CBF_Convex_Reformulation_Final} where $\epsilon$ is taken small enough such that $k = 1$:
\begin{align}
\label{eq: CBF_Convex_Reformulation_QP_Special}
& \min_{\ubfu \in \underline{\calU}}\,\, \|L(\bfx)^\top(\ubfu - \tilde{\underline{\bfk}}(\bfx))\|^2  \notag \\
\mathrm{s.t.} \, \,  
& r_2 L_F(\ubfu) - \epsilon \textit{CBC}_1  \leq 0. 
\end{align}
Note that to make \eqref{eq: CBF_Convex_Reformulation_QP_Special} a QP we need to make $L_F(\ubfu) = \|\ubfu^\top \bfR(\bfx)\|_{\infty}$.
The following mix-integer problem is used to obtain $\textit{CBC}_1$:
\begin{align}
\label{eq: mixint_max_CBC}
& \textit{CBC}_i - M(1-z_i) \leq t \leq \textit{CBC}_i, \notag \\
& \sum_{i=1}^N z_i = 1, \ z_i \in \{ 0,1 \}, M>>1.
\end{align}
However, for a more general case $k = \lceil N\epsilon \rceil > 1$, it is more complicate to solve:
\begin{proposition}
	\label{proposition: CBF_Convex_Reformulation_QP_General}
	If every assumptions in \ref{proposition: CBF_Convex_Reformulation_QP_Special} holds excepts: $k = \lceil N\epsilon \rceil > 1$, the optimization problem \eqref{eq: CBF_Convex_Reformulation_Final} can be reformulated equivalently as the following Min-integer QP, 
	\begin{align}
	\label{eq: CBF_Convex_Reformulation_QP_General_Final}
	& \min_{\ubfu \in \underline{\calU}}\,\, \|L(\bfx)^\top(\ubfu - \tilde{\underline{\bfk}}(\bfx))\|^2  \notag \\
	\mathrm{s.t.} \, \,
	& | \ubfu^\top \bfR(\bfx) | \leq \mathbf{1}_{dim(\bfxi)} \otimes (\frac{\epsilon}{r_2} t - \frac{1}{N r_2}\sum_{i=1}^N s_i), \notag\\
	& -q(\ubfu) + t - \ubfu^\top \bfR(\bfx) \bfxi_i \leq s_i, \ s_i \geq 0, \notag \\
	& -q(\ubfu) + t - \ubfu^\top \bfR(\bfx) \bfxi_i \geq \bar{s}_i, \ \bar{s}_i \leq 0, \notag \\
	& s_i \leq Mz_i, \ z_i \in \{ 0,1 \}, M>>1, \notag \\
	& -\bar{s}_i \leq M\bar{z}_i, \ \bar{z}_i \in \{ 0,1 \}, \notag \\
	& q(\ubfu) - t + \ubfu^\top \bfR(\bfx) \bfxi_i + s_i \leq M(1-z_i), \notag \\
	& -q(\ubfu) + t - \ubfu^\top \bfR(\bfx) \bfxi_i - \bar{s}_i \leq M(1-\bar{z}_i), \notag \\
	& s_i \leq M\zeta_i, -\bar{s}_i \leq M\bar{\zeta}_i, \zeta_i \in \{ 0,1 \}, \bar{\zeta}_i \in \{ 0,1 \}, \notag \\
	& \nu_i \leq M(1-\zeta_i), \bar{\nu}_i \leq M(1-\bar{\zeta}_i), \nu_i \in \{ 0,1 \}, \bar{\nu}_i \in \{ 0,1 \}, \notag \\
	& \sum_{i=1}^N \nu_i = N+1-k, \ \sum_{i=1}^N \bar{\nu}_i = k.
	\end{align}
\end{proposition}

\subsection{Robust Formulation of CBC} In this section we want to find a lower bound $\textit{CBC}_{robust}$ on equation \eqref{eq: cbc_kronecker}, i.e., $ \textit{CBC}(\bfx,\ubfu,\bfxi) \geq \textit{CBC}_{robust}$. We have: $\textit{CBC}(\bfx,\ubfu,\bfxi) = q(\ubfu) + \ubfu^T\bfR(\bfx)\bfxi$ and thus:
\begin{equation} \label{eq: robust_nonseperate}
	q(\ubfu) + \ubfu^T\bfR(\bfx)\bfxi \geq q(\ubfu) - \| \ubfu^T\bfR(\bfx)\bfxi \|, \ \forall \bfx, \ubfu, \bfxi.
\end{equation}
Further, we want to separate $\bfxi$ from the expression above, to achieve this, we need to find an upper bound of $\| \ubfu^T\bfR(\bfx)\bfxi \|$, which is:
\begin{equation} \label{eq: robust_upperxi}
	\| \ubfu^T\bfR(\bfx) \|_p \| \bfxi \|_q \geq \| \ubfu^T\bfR(\bfx)\bfxi \|, \ \frac{1}{p} + \frac{1}{q} = 1, \ \forall \bfx, \ubfu, \bfxi.
\end{equation}
Above all, we have obtained the following expression for $\textit{CBC}_{robust}$:
\begin{equation} \label{eq: cbc_robust}
	\textit{CBC}_{robust} = q(\ubfu) - \| \ubfu^T\bfR(\bfx) \|_p \| \bfxi \|_q.
\end{equation}
As a result, if we could find $\ubfu$ such that $\textit{CBC}_{robust} \geq 0$, then we will have $\textit{CBC}(\bfx,\ubfu,\bfxi) \geq 0$.
Now consider our convex approximation of the DRCCP problem with $\epsilon \leq \frac{1}{N}$, we will have the following constraint on CBC:
\begin{equation} \label{eq: cbc_convex_special_ori}
	\frac{r_2}{\epsilon} L_F(\ubfu) - \min_{\bfxi \in \Xi_N} \textit{CBC}  \leq 0.
\end{equation}
where $\Xi_N$ denote the set our samples of $\bfxi$. If we define $L_F(\ubfu) := \|\ubfu^\top \bfR(\bfx)\|_{p}$, then we will find that:
\begin{equation} \label{eq: cbc_convex_special_fin}
	\frac{r_2}{\epsilon} \|\ubfu^\top \bfR(\bfx)\|_{p} - q(\ubfu) - \min_{\bfxi \in \Xi_N} \ubfu^T\bfR(\bfx)\bfxi  \leq 0.
\end{equation}
which took the similar form as our robust formulation.
