# Supplementary material for: Safe and Stable Control Synthesis for Uncertain System Models via Distributionally Robust Optimization
Source: arXiv:2210.01341 source file (2023-03-16)
Supplement: Supplementary file 2 [file Appendix_Prop41.tex]

\section{Original Convex MIQP Reformulation}

\begin{proposition}
\label{proposition: convex_final_miqp_appdx}
Given the expression of $G_l$ in \eqref{eq: G_def}, consider the $p$-Wasserstein distance with $p=1$ and suppose $\Xi = \bbR^{k}$, the following mixed-integer quadratic program (MIQP) is equivalent to \eqref{eq: general_control_synthesis},
\begin{align}
\label{eq: CBF_Convex_final_appdx}
& \min_{\ubfu \in \underline{\calU}, t \in \bbR, s_i \in \bbR, z_i}\,\, \|\ubfu - \underline{\bfk}(\bfx)\|^2  \\
\mathrm{s.t.} \, \,  
& r L(\ubfu, \bfx) + \frac{1}{N} \sum_{i=1}^{N} s_i - t \epsilon \leq 0, \notag  \\
& s_i \geq G_l(i)+t, \; \; s_i \geq 0,  \notag \\
& s_i \leq G_l(i)+t +Mz_i, \; \; s_i \leq M(1-z_i), \notag \\
&z_i \in \{0,1 \}, \quad M \gg 1, \quad i = 1,2,\dots N. \notag
\end{align}
\end{proposition}
\begin{proof}
We start by considering the following program:
\begin{align}
\label{eq: CBF_Convex_Reformulation_appdx}
& \min_{\ubfu \in \underline{\calU}}\,\, \|\ubfu - \underline{\bfk}(\bfx)\|^2\\
\mathrm{s.t.} \, \,  
& r L(\ubfu, \bfx) + \inf_{t \in \mathbb{R}}\left[\frac{1}{N} \sum_{i=1}^{N} (G_l(i) + t)_+ - t \epsilon\right] \leq 0. \notag  
\end{align}
Based on \cite[Lemma V.8]{Hota2019DataDrivenCC} and assuming $\Xi = \bbR^k$, the supremum over
the Wasserstein ambiguity set (the constraint in \eqref{eq: general_control_synthesis}) can be written equivalently as the sample average $\inf_{t \in \mathbb{R}}\left[\frac{1}{N} \sum_{i=1}^{N} (G_l(i) + t)_+ - t \epsilon\right]$ and a regularization term $r L(\ubfu, \bfx)$. This implies that \eqref{eq: CBF_Convex_Reformulation} is equivalent to \eqref{eq: general_control_synthesis}. 
% Note that the constraint in \eqref{eq: CBF_Convex_Reformulation} is the sample average 
To enable online controller synthesis, we further consider reformulating the bi-level optimization \eqref{eq: CBF_Convex_Reformulation} to the following program:
\begin{align}
\label{eq: CBF_Convex_remove_inf_appdx}
& \min_{\ubfu \in \underline{\calU}, t \in \bbR}\,\, \|\ubfu - \underline{\bfk}(\bfx)\|^2  \\
\mathrm{s.t.} \, \,  
& r L(\ubfu, \bfx) + \frac{1}{N} \sum_{i=1}^{N} (G_l(i) + t )_+ - t \epsilon \leq 0. \notag
\end{align}
%
% \marginJC{If (22) is equivalent to (21), and (21) is equivalent to (19), why don't we remove the middle man, eliminate Lemma IV.1, and directly state the proposition? The proof of Prop IV.2 can contain the formulation (21), where we refer to [20, Lemma V.8].}
%
We next show \eqref{eq: CBF_Convex_remove_inf_appdx} is equivalent to \eqref{eq: CBF_Convex_Reformulation_appdx}. Let $(\ubfu_1, t^*)$ denote an optimal solution to \eqref{eq: CBF_Convex_remove_inf_appdx} and $\ubfu_2$ an optimal solution to \eqref{eq: CBF_Convex_Reformulation_appdx}, with $\hat{t}$ the optimizer for the $\inf$ terms in the constraint of \eqref{eq: CBF_Convex_Reformulation_appdx}.
Given $(\ubfu_1, t^*)$, we have
\begin{align*}
    &r L(\ubfu_1, \bfx) + \frac{1}{N} \sum_{i=1}^{N} (G_l(i) + t^*)_+ - t^* \epsilon \leq 0,
\end{align*}
which implies the constraint in \eqref{eq: CBF_Convex_Reformulation} is satisfied. 
%
% \begin{equation*}
%     r_2 L_h(\ubfu_1) + \inf_{t \in \mathbb{R}}\left[\frac{1}{N} \sum_{i=1}^{N} (-\textit{CBC}_i + t)_+ - t \epsilon\right] \leq 0. 
% \end{equation*}
%
This implies that $\ubfu_1$ is also a solution to \eqref{eq: CBF_Convex_Reformulation}, and the cost satisfies $\|L(\bfx)^\top(\ubfu_1 - \tilde{\underline{\bfk}}(\bfx))\|^2 \geq \|L(\bfx)^\top(\ubfu_2 - \tilde{\underline{\bfk}}(\bfx))\|^2 $.

% \NA{More precisely $\ubfu_1$ is feasible in \eqref{eq: CBF_Convex_Reformulation} and its cost satisfies $\|L(\bfx)^\top(\ubfu_1 - \tilde{\underline{\bfk}}(\bfx))\|^2 \geq \|L(\bfx)^\top(\ubfu_2 - \tilde{\underline{\bfk}}(\bfx))\|^2$, where $\ubfu_2$ is an optimal solution to \eqref{eq: CBF_Convex_Reformulation}. Introduce $(\ubfu_1, t_1)$ and $(\ubfu_2, t*)$ in the very beginning of the proof and show the cost relationship in addition to feasibility in the if and only if parts of the proof.}. 

Given $\ubfu_2$ and $\hat{t}$, we have
\begin{align*}
    &r L(\ubfu_2, \bfx) + \frac{1}{N} \sum_{i=1}^{N} (G_l(i) + \hat{t} )_+ - \hat{t} \epsilon \leq 0,
\end{align*}
which implies $(\ubfu_2,\hat{t})$ is also a solution to \eqref{eq: CBF_Convex_remove_inf_appdx}. Furthermore, the cost satisfies $\|L(\bfx)^\top(\ubfu_1 - \tilde{\underline{\bfk}}(\bfx))\|^2 \leq \|L(\bfx)^\top(\ubfu_2 - \tilde{\underline{\bfk}}(\bfx))\|^2  $ since $(\ubfu_1, t^*)$ is the optimal solution to \eqref{eq: CBF_Convex_remove_inf_appdx}. Therefore, both costs are equal, and \eqref{eq: CBF_Convex_remove_inf_appdx} and \eqref{eq: CBF_Convex_Reformulation_appdx} are equivalent.

We rewrite the ReLU term $(G_l(i)+t)_+$ equivalently as the following mixed-integer inequalities:
\begin{align}
\label{eq: relu_reformulate_appdx}
    &s_i \geq G_l(i)+t, \quad s_i \geq 0, \quad s_i \leq M(1-z), \\
    &s_i \leq G_l(i)+t + Mz,  \quad z \in \{0,1\}, \quad M \in \bbR, \quad M \gg 1. \notag
\end{align}
Note that the mixed-integer reformulation is valid only if $M \geq G_l(i) + t$. We thus set $M$ large in practice since we do not know the explicit value of $G_l(i) + t$ when solving the program. From \eqref{eq: CBF_Convex_remove_inf_appdx} and \eqref{eq: relu_reformulate_appdx}, we conclude that \eqref{eq: CBF_Convex_final_appdx} is equivalent to \eqref{eq: general_control_synthesis}.

\end{proof}
