# Supplementary material for: Safe and Stable Control Synthesis for Uncertain System Models via Distributionally Robust Optimization
Source: arXiv:2210.01341 source file (2023-03-16)
Supplement: Supplementary file 3 [file Appendix_relu.tex]

\section{Mixed Integer Reformulation of ReLU}\label{}

% \NA{This lemma is just a couple of lines. Since there is nothing else in the Appendix, perhaps it can be moved where it is needed in the main text.}
% \begin{lemma}
% \label{lemma: reformulate_relu_mixed_integer}
% A ReLU equality $y = (x)_+$ can be reformulated equivalently as the following mixed-integer inequalities:
% %
% \begin{align}
%     &y \geq x, \quad y \geq 0, \quad y \leq M(1-z), 
%     \quad y \leq x + Mz, \notag \\ 
%     &z \in \{0,1\}, \quad M \gg 1. \notag
% \end{align}
% \end{lemma}

%
\begin{table} 
	\centering
	%\captionsetup{font={scriptsize}} \caption{Failure rate and average CBF values of the ACC simulation results. The results are shown in the following format: $a\% \mid b$, where $a\%$ denotes the violation rate of each formulation: (simulations with unsafe state)/(total simulations), and $b$ denotes the average value of CBF over all simulations. Average CBF value is computed based on stabilized CBF values (e.g. $5 \leq t \leq 15$ in Figure~\ref{fig: out_of_support}).} 
	%\KL{Add more explanations for the table}
	\scalebox{0.7}{
    \begin{tabular}{cccccc}
		\toprule 
		Case & \begin{tabular}{c}Convex \\ DRCCP \end{tabular}& \begin{tabular}{c}Affine \\ DRCCP \end{tabular} &  \begin{tabular}{c}Robust \\ CLF-CBF-SOCP \end{tabular} & \begin{tabular}{c}Gaussian \\ CLF-CBF-SOCP \end{tabular} & \begin{tabular}{c}Original \\ CLF-CBF-QP \end{tabular} \\
		\midrule  
		1 & 0\% $\mid$ 2.11 & $\boldsymbol{0\%}$ $\mid$ $\bf0.56$ & 0\% $\mid$ 1.01 & 0\% $\mid$ 0.55 & 100\% $\mid$ -0.48 \\
        2 & $\boldsymbol{0\%}$ $\mid$ $\bf0.35$ & $\boldsymbol{0\%}$ $\mid$ $\bf0.35$ & 0\% $\mid$ 1.01 & 0\% $\mid$ 0.56 & 100\% $\mid$ -0.48 \\
		3 & 0\% $\mid$ 1.23 & $\boldsymbol{0\%}$ $\mid$ $\bf0.55$ & 0\% $\mid$ 0.96 & 98\% $\mid$ -0.17 & 100\% $\mid$ -0.50 \\
		4 & 0\% $\mid$ 0.56 & $\boldsymbol{0\%}$ $\mid$ $\bf0.51$ & 0\% $\mid$ 0.89 & 100\% $\mid$ -0.92 & 100\% $\mid$ -0.53 \\
		5 & 0\% $\mid$ 1.42 & $\boldsymbol{0\%}$ $\mid$ $\bf0.57$ & 0\% $\mid$ 1.01 & 100\% $\mid$ -0.88 & 100\% $\mid$ -0.48 \\
		6 & 0\% $\mid$ 1.94 & $\boldsymbol{0\%}$ $\mid$ $\bf0.57$ & 0\% $\mid$ 1.01 & 100\% $\mid$ -0.65 & 100\% $\mid$ -0.48 \\
		7 & 0\% $\mid$ 4.49 & $\boldsymbol{0\%}$ $\mid$ $\bf0.57$ & 0\% $\mid$ 1.01 & 100\% $\mid$ -0.64 & 100\% $\mid$ -0.49 \\
		8 & $\boldsymbol{0\%}$ $\mid$ $\bf1.29$ & 98\% $\mid$ -0.26 & 84\% $\mid$ -0.16 & 100\% $\mid$ -0.57 & 100\% $\mid$ -0.51 \\
		\bottomrule
	\end{tabular}}
	\label{table: results_new}
\end{table}
